# Supplementary material for: Eye of the Beholder: Towards Measuring Visualization Complexity
Source: arXiv:2512.05536 source file (2025-12-05)
Supplement: Supplementary file 1 [file appendix_A.tex]

\section{Experiment Reporting Form}
\label{appx:a}

Adapted from Borgo et al.~\cite{borgo_information_2018}

% Icons require the fontawesome5 package: 
% \usepackage{fontawesome}
%\begin{table*}[!h]
%\centering
\noindent
\begin{tabular}{p{3.1cm}|p{13.3cm}}
\toprule
\textbf{Study:}         &  Visualization Complexity Rating using crowdsourcing \\
\textbf{Experiment:}    &  1 -- Rate the complexity of the presented visualization and give a reason for why this rating \\ \midrule
Study Design            &  Type: \faIcon[regular]{circle} ~ between-subject \hspace{1cm} \faIcon[regular]{check-circle}  ~ within-subject    \hspace{1cm} \faIcon[regular]{circle} ~ mixed-design, with \newline 
                           \textit{Independent Variables:} Visualization \newline 
                           \textit{Dependent Variables:} Perceived complexity score of the visualization reported on a likert scale [1..10] \newline 
                           \textit{Covariates:} Experience with visualizations, educational level
\\ \midrule
Experiment Data         &  \textit{Source:} Dataset of online visualizations used in \cite{DBLP:journals/tvcg/ShinCHE23} \newline 
                           \textit{Specifics:} 640 visualizations scraped from the web in jpg format. \newline
                           \textit{Variations:} 50 visualization types, not evenly distributed in the dataset. 
\\ \midrule
Task                    &  \textit{Elementary:} Qualitative estimation and reflection \textit{Synoptic:} n/a \textit{Mixed:} n/a \newline 
                           \textit{Variations:} n/a
\\ \midrule
Visualizations          &  \textit{Type:}  \faIcon[regular]{check-circle} ~ static \hspace{1cm} \faIcon[regular]{circle} ~ interactive    \hspace{1cm} \faIcon[regular]{circle} ~ other \newline 
                           \textit{Specifics:} 640 visualizations in jpg format, covering 50 visualization types, not evenly distributed throughout the dataset. Visualizations are of varying size, design and quality. 
\\ \midrule
Test Question Format    &  \textit{Questions asked:} Qualitative estimation question for a given visualization + reflection on the chosen estimation. \newline 
                           \textit{Response type:} Likert scale, and user-creatable tag-picker\newline
                           \textit{Associated data, task, visualizations:} 2 questions X 50 visualizations per participant. 
\\ \midrule
Participants            &  \textit{Expected number per independent variable:} 300      \hspace{1cm} \textit{in total:} 289 \newline 
                           \textit{Requisites:} Fluency in English, 50\% male/female quota enforced. 
\\ \midrule
Quality Measures        &  \textit{Attention detectors:} n/a \newline 
                           \textit{Multiple participation:} Multiple participations were prohibited via the crowdsourcing platform (Prolific) \newline 
                           \textit{Others:} n/a
\\ \midrule
Motivations             &  \textit{Intrinsic:} n/a \newline 
                           \textit{Extrinsic:} £8.92/hr. Median completion time of 32 minutes equals £4.83 in reward. 
\\ \midrule
System Requirements     &  \textit{Hardware:}  Tablet, laptop or desktop computer. Smartphones were excluded. \newline 
                           \textit{Software:}  Javascript enabled in web browser. 
\\ \midrule
Procedure               &  \textit{Training:} 7 examples visualizations \newline 
                           \textit{Dummy questions (not in training):} n/a \newline 
                           \textit{Test questions number per participant:}    7   \hspace{1cm} \textit{ordering:} Same order for each participant. \newline 
                           \textit{Quality assurance questions:}  n/a   \newline 
                           \textit{Ability test:} n/a \newline 
                           \textit{Questionnaires:} 1 demographics questionaire \newline 
                           \textit{Steps:} 1 introduction; 2 consent; 3 demographics form; 4 task instruction; 5 task setup; 6 training questions; main task (50 X visualizations); 7 thank you note
\\ \midrule
Data Collection         &  \textit{Method:} Participants filled in the questions on screen for each visualization stimuli. \newline 
                           \textit{Managed by:}  ReVISit tool with Google Firebase integration   \hspace{1cm} \textit{Time Period:} Aug 2024 \newline 
                           \textit{Testing before actual study:} 2 rounds of pilot studying, each with 2 participants. 
\\ \midrule
Collected Data Analysis &  \textit{Average experiment length:} 32 mins \newline 
                           \textit{Number of participants (before filtering):} 625\newline 
                           \textit{Excluded participants        with low quality data:}    4      \hspace{1cm} \textit{for other reasons:}   332 (305 left the study, 27 timed out)  \hspace{1cm} \textit{in total:} 336 \newline 
                           \textit{Included participants        per independent variable:}        289      \hspace{1cm} \textit{in total:} 289 \newline 
                           \textit{Included participants' demographics:}  50\% female; mean age = 30; 53\% Europeans, 38\% Africans, 4\% North Americans, 120 from South Africa, 35 from Portugal, 34 from Poland; 30\% with bachelor's degree, 77\% bachelor's degree or lower \newline 
                           \textit{Statistics methods used:} t-tests in the follow-up experiments.
\\ \midrule
Reproducibility         &  \textit{Experiment Material:} dataset, task, and ReVISit source code available at [[link]] \newline 
                           \textit{Collected (Anonymized) Data:} All collected anonymized data is available at [[link]]
\\ \bottomrule
\end{tabular}
%\caption{}
%\label{tab:my-table}
%\end{table*}
